# Supplementary material for: Cascaded Multiparameter Quantum Metrology
Source: arXiv:2304.08545 ancillary file (2025-01-17)
Supplement: Supplementary file 1 [file SI_V5e_New_cascaded_Architecture.pdf]

# Supplemental Material: New Cascaded Architecture for Classical and Quantum Multiparameter Sensing

Gregory Krueper,<sup>1</sup> Lior Cohen,<sup>2</sup> and Juliet T. Gopinath<sup>1,2</sup>

*Department of Physics, University of Colorado Boulder, Boulder CO 80309, USA*

*Department of Electrical, Computer and Energy Engineering,*

*University of Colorado Boulder, Boulder CO 80309, USA*

## Calculating the unitary matrix

Constructing the unitary matrix for a sensor requires some accounting of the number of temporal modes  $M$  in the system. The total number of modes will be:

$$M = (k + 1)(N - 2) + m \quad (1)$$

Where  $N$  is the number of phases,  $k$  is the number of reflections each temporal mode can undergo, and  $m$  is the number of input pulses.

A series of beamsplitter (reflector) and phase shift operations map  $M$  input modes onto  $M$  output modes in a  $2M \times 2M$  unitary matrix. Figure 1 helps visualize this map for an example with four phases and 6 modes. Each phase shift operation  $\hat{P}(\phi)$  is a sub-matrix:

$$\hat{P}(\phi) = \begin{pmatrix} \cos(\phi) & -\sin(\phi) \\ \sin(\phi) & \cos(\phi) \end{pmatrix} \quad (2)$$

which starts on the  $2n$ -th diagonal element for mode  $n$ . All other diagonal entries are 1 and all other off-diagonal entries are 0. Each beamsplitter sub-matrix  $\hat{B}(T)$  is:

$$\hat{B}(T) = \begin{pmatrix} \sqrt{T} & 0 & \cdot & \sqrt{1-T} & 0 \\ 0 & \sqrt{T} & \cdot & 0 & \sqrt{1-T} \\ \cdot & \cdot & \cdot & \cdot & \cdot \\ -\sqrt{1-T} & 0 & \cdot & \sqrt{T} & 0 \\ 0 & -\sqrt{1-T} & \cdot & 0 & \sqrt{T} \end{pmatrix} \quad (3)$$

The matrix couples modes two different modes with transmission  $T$ . The dots indicate that the identity matrix should be inserted there if these modes are not adjacent. There are many ways to represent a beamsplitter matrix for Gaussian operations, but this one proved most convenient. Since the paths of temporal modes have both transmission and reflection, one should instead input  $1 - T$  to represent a reflective operation. For example, in Figure 1, the reflection for input mode 1 at time  $t_1$  would be transmissive, while at time  $t_3$  it would be reflective. The unitary is then a multiplication of phase shifts and beamsplitter operations for each active mode at each time, where phase shifts act before beamsplitters.

For truncation due to finite reflections, the final two modes (1 and 2 in the present example) undergo a loss transformation. This is described by equation 3 in which only the affected modes have  $\mathbf{U} = \sqrt{T}\mathbf{I}$ , where  $\mathbf{I}$  is the identity matrix,  $\vec{d} = 0$ , and  $\mathbf{Y} = (1 - T)\mathbf{I}$ .

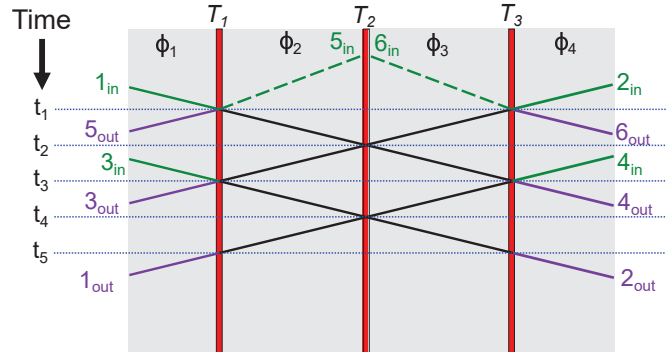

FIG. 1. A visualization for the construction of the unitary matrix of the sensor, similar to figure 1(b). In this example of a four-phase sensing arm, each temporal mode is tracked through each of its phase shift and reflection operations, shown as a function of time. By tracking  $k = 1$  reflections, six output temporal modes are mapped to six input temporal modes, including two inaccessible vacuum modes.

## Optical loss and added noise

Of course, the sensor does not infinitely scale to an arbitrarily high number of phases. For a meaningful quantum advantage, the number of input phase-locked squeezed pulses scales alongside  $N$ , which may become experimentally challenging. Additionally, dispersion, optical loss, and limited coherence will all set an upper limit on the number of optical elements that the squeezed pulses pass through. Dispersion can coherence can be engineered, but optical loss sets a harder limit.

Using the above treatment for optical loss, we analyzed the extent to which the sensor can maintain a quantum advantage under lossy conditions. Results are in Figure 2(a). A non-unity efficiency introduces added noise into the state, effectively reducing the squeezing strength and the resulting quantum advantage  $Q$ . Similarly, we analyzed how added thermal noise or phase noise affects  $Q$ . Mixing the output state with a thermal state of average photon number  $n_{th}$  reduces  $Q$  as shown in 2(b).

## Multiparameter estimation advantage

The quantum-enhanced multiparameter estimation from Figure 4 may also be compared with that of individual phase estimation in a series of three separate measurements. Figure 3 shows three traces of the opti-

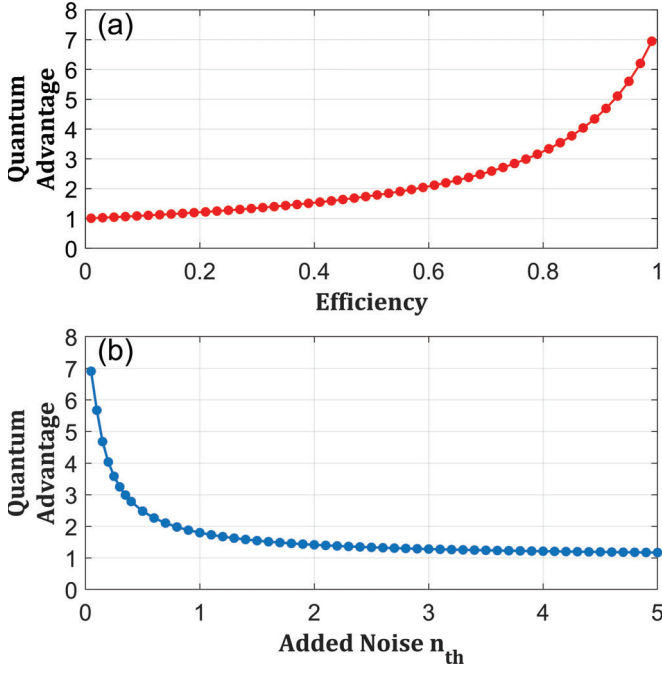

FIG. 2. Results showing the degradation in quantum advantage of the sensor as one adds (a) optical loss, and (b) thermal noise, described by an average number of thermal photons  $n_{th}$ . Loss effectively reduces the squeezing strength. Added thermal noise ruins the condition of having a shot-noise limited system, without which squeezing is ineffective.

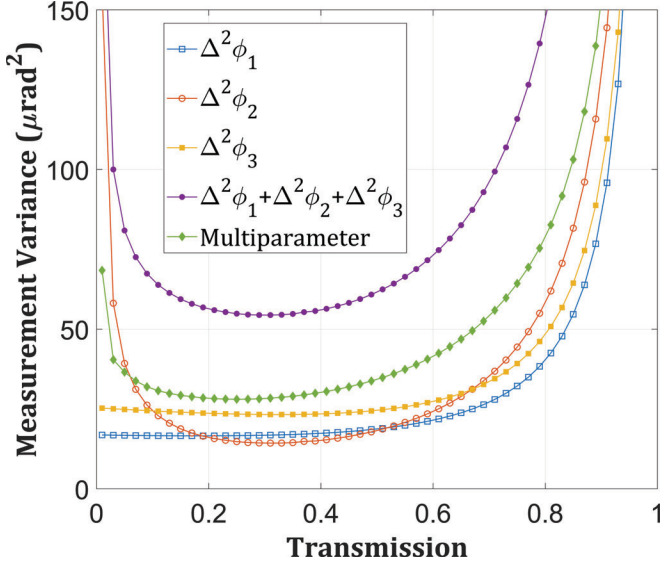

FIG. 3. A comparison of measurement sensitivities from different methods in the three-phase interferometer, as a function of reflector transmission. The traces for phases 1, 2, and 3 refer to single-parameter estimation of those phases, assuming the others are known. The sum of those traces as three separate measurements is compared with the total variance from measuring all phases at once in a multiparameter approach. The total phase variance from a multiparameter estimation is shown to be between 1.7 and 2.8 lower than that of sensing individual phases, showing the efficacy of sensing all parameters at once.

mal variance for measuring each phase individually using 5 pulses, multiplied by 3 because each phase is measured one third as often. The sum of these variances is also plotted, and compared to that of multiparameter estimation, where the total phase variance was optimized collectively. The total variance of the multiparameter measurement is between 1.7 and 2.8 times lower than the sum of individual measurements. This lower variance shows a separate advantage of using multiparameter estimation techniques, on top of using squeezed light.
